# Supplementary material for: Using Multiple Instance Learning to Build Multimodal Representations
Source: arXiv:2212.05561 source file (2023-03-09)
Supplement: Supplementary file 1 [file supp.pdf]

# Supplementary

No Author Given

No Institute Given

## 1 Permutation-Invariant Score Functions: Revisited

**Table 1.** The bag score function $S$ is constructed from aggregators $\pi, \pi_s$ and instance or bag classifiers $h, g$. We restrict $h, g$ to be identity or cosine similarity.

| Approach | $h$ | $\pi$ | $g$ | $\pi_s$ |
|---|---|---|---|---|
| Local | $\mathcal{X} \times \mathcal{Y} \to \mathbb{R}$ | $\mathcal{P}(\mathbb{R}) \times \mathcal{Y} \to \mathbb{R}$ | Identity | $\mathcal{P}(\mathbb{R}) \to \mathbb{R}$ |
| Global | Identity | $\mathcal{P}(\mathcal{X}) \times \mathcal{Y} \to \mathcal{X}$ | $\mathcal{X} \times \mathcal{Y} \to \mathbb{R}$ | $\mathcal{P}(\mathbb{R}) \to \mathbb{R}$ |

In this section, we directly extend the classifier formulation in [7] to contrastive representation learning where the formulation in Section 2.2 becomes a special case. We use roughly the same notation as those introduced in Section 2 with minor modifications. In particular, we use $\{x_n\}$ where $x_n \in \mathcal{X}$ to denote the input bag of features and $\{y_m\}$ where $y_m \in \mathcal{Y}$ to denote the set of label features.

We propose a simple recipe for building a permutation-invariant bag score function via the composition of the following functions: (i) a transformation of instances $h$, (ii) a permutation invariant function $\pi$ that combines the transformed instances, (iii) a transformation of the combined instances $g$ and (iv) a permutation invariant function $\pi_s$ that combines the input bag score for each label in the label bag. In summary, we model the bag score function $S$ as

$$S\left(\{x_n\}, \{y_m\}\right) = \pi_s\left(\left\{g\left(\pi\left(\{h(x_n, y_m)\}_n, y_m\right), y_m\right)\right\}_m\right). \quad (1)$$

For finite number of classes, the score function can simply output the scores for every class. This becomes unwieldy for labels with infinite number of possibilities, e.g., sentence features. Instead, the transformations $h, \pi, g$ can potentially rely on the label features $y_m$ to multiplex the transformation.

As shown in Table 1, There are two main approaches, local and global, to construct the bag score function, depending on the functional forms of $h, \pi, g, \pi_s$. Equation 1 subsumes the formulation in Section 2.2. In the local approach, the bag score is induced by aggregating the instance scores. The instance classifier $h$ scores the instance features conditioned on the bag label features. All $M$ label specific bag scores are aggregated via $\pi$ from the instance scores without further processing by $g$. Finally, the bag score is aggregated via $\pi_s$ from the label-specific bag scores. In the global approach, the bag score is computed from

**Table 2.** Taxonomy of multimodal representation learning methods under our bag score function framework. Previous works use different approaches, operate on data at varying scales, and employ a range of instance aggregators. Under L/G column, we use L and G to denote local and global approach. Under $x_n$ and $y_m$ columns, we list what $x_n$ and $y_m$ represent. We use $i, r, w, s, a, v$ to denote image, image region, word, sentence, audio, and video respectively. Let $h = \{h_n\}$ be instances and $A$ be aggregator, e.g., $\pi$ or $\pi_s$, with implicit dependence on $w$, the label features, i.e., $A(h) = \pi(\{h_n\}, w)$. Under $\pi$ and $\pi_s$ columns, we denote $A(h) = \sum_n \alpha_n h_n$ where $\alpha_n = \exp(h_n \cdot w) / \sum_m \exp(h_m \cdot w)$ as cross attention, $A(h) = \frac{1}{N} \sum_n h_n$ as average, $A(h) = \sum_n h_n$ as sum, $A(h) = \sum_n h_n$ as max, $A(h) = \log \sum_n \exp(t \cdot h_n)/t$ as $\text{LSE}_t$, $A(\{h\}) = h$ as identity, Equation 4 as Non-Local, any nonlinear network as NN. We use n. and d. to mean numerator and denominator of the contrastive loss.

| Methods | L/G | $x_n$ | $y_m$ | $\pi$ | $\pi_s$ |
|---|---|---|---|---|---|
| NeuralTalk [8] | L | r | w | Max | Sum |
| DAVEnet-MISA [5] | L | r | a | Max | Sum |
| MIML [3] | L | v | a | Max | Max |
| Info-Ground [4] | G | r | w | Cross Attention | n. Sum; d. $\text{LSE}_1$ |
| MIL-NCE [9] | G | v | s | Average | $\text{LSE}_1$ |
| ConVIRT/CLIP [11, 10] | G | r | s | NN $\circ$ Avearge | Identity |
| GLoRIA/BioViL [6, 1] | L | r | w | Cross Attention | $\text{LSE}_t$ |
| | G | r | s | Average | Identity |
| Ours | L | r | s | $\text{LSE}_t$ | Sum |
| | G | r | s | Non-Local | Sum |

a bag feature that is aggregated from the instance features. Again, $\pi_s$ is the bag score aggregation function with respect to each label in the label bag.

In both approaches, $g, h$ are fixed and $\pi, \pi_s$ are the degree of freedom in modeling the bag score function $S$. As we will see empirically, the aggregation function $\pi$ heavily impacts the performance on downstream tasks.

Quite a few representation learning methods listed in Table 2 are special cases of this framework. We want to emphasize that these prior approaches restrict the bag score function to be permutation-invariant, even if this assumption is not explicitly articulated. As an example, NeuralTalk [8] is a local approach where the bag score is obtained by first computing the max instance scores with respect to the image regions for each phrase in the caption followed by summing up phrase-specific bag scores. In Table 2, the instances and the labels may represent entities at varying scales. For example, CLIP [11, 10] contrast whole image and sentences and therefore $\{y_m\}$ is a set with cardinality of one containing the sentence feature. In comparison, GLoRIA contrast image regions and words so $\{y_m\}$ is a set of words. We observe a diverse set of aggregators $\pi, \pi_s$ over instances and labels at different scales, implying there may be not a single set of aggregators that works well for every problem. More realistically, the best instance aggregators are ones that fit application-specific assumptions well.

We acknowledge there are additional ways to construct $S$ that we will not investigate further in this paper. For example, [2] applies aggregates region and word features to obtain the input bag features for the entire label bag.

## References


1. Boecking, B., Usuyama, N., Bannur, S., Castro, D.C., Schwaighofer, A., Hyland, S., Wetscherek, M., Naumann, T., Nori, A., Alvarez-Valle, J., Poon, H., Oktay, O.: Making the Most of Text Semantics to Improve Biomedical Vision–Language Processing (Jul 2022)
2. Datta, S., Sikka, K., Roy, A., Ahuja, K., Parikh, D., Divakaran, A.: Align2Ground: Weakly Supervised Phrase Grounding Guided by Image-Caption Alignment. In: 2019 IEEE/CVF International Conference on Computer Vision (ICCV). pp. 2601–2610. IEEE, Seoul, Korea (South) (Oct 2019). https://doi.org/10.1109/ICCV.2019.00269
3. Gao, R., Feris, R., Grauman, K.: Learning to Separate Object Sounds by Watching Unlabeled Video (Jul 2018)
4. Gupta, T., Vahdat, A., Chechik, G., Yang, X., Kautz, J., Hoiem, D.: Contrastive Learning for Weakly Supervised Phrase Grounding (Aug 2020)
5. Harwath, D., Recasens, A., Surís, D., Chuang, G., Torralba, A., Glass, J.: Jointly Discovering Visual Objects and Spoken Words from Raw Sensory Input. arXiv:1804.01452 [cs] (Apr 2018)
6. Huang, S.C., Shen, L., Lungren, M.P., Yeung, S.: GLoRIA: A Multimodal Global-Local Representation Learning Framework for Label-Efficient Medical Image Recognition p. 10 (2021)
7. Ilse, M., Tomczak, J.M., Welling, M.: Attention-based Deep Multiple Instance Learning. arXiv:1802.04712 [cs, stat] (Jun 2018)
8. Karpathy, A., Fei-Fei, L.: Deep Visual-Semantic Alignments for Generating Image Descriptions (Apr 2015)
9. Miech, A., Alayrac, J.B., Smaira, L., Laptev, I., Sivic, J., Zisserman, A.: End-to-End Learning of Visual Representations From Uncurated Instructional Videos. In: 2020 IEEE/CVF Conference on Computer Vision and Pattern Recognition (CVPR). pp. 9876–9886. IEEE, Seattle, WA, USA (Jun 2020). https://doi.org/10.1109/CVPR42600.2020.00990
10. Radford, A., Kim, J.W., Hallacy, C., Ramesh, A., Goh, G., Agarwal, S., Sastry, G., Askell, A., Mishkin, P., Clark, J., Krueger, G., Sutskever, I.: Learning Transferable Visual Models From Natural Language Supervision. arXiv:2103.00020 [cs] (Feb 2021)
11. Zhang, Y., Jiang, H., Miura, Y., Manning, C.D., Langlotz, C.P.: Contrastive Learning of Medical Visual Representations from Paired Images and Text (Sep 2022)
